# Supplementary material for: Improved Outlier Robust Seeding for k-means
Source: arXiv:2309.02710 source file (2023-09-06)
Supplement: Supplementary file 1 [file appendix.tex]

\newpage
\appendix
\section{Appendix}
\subsection{Result on Real world datasets}
\subsubsection{Results on~\texttt{Shuttle} dataset} 
\texttt{Shuttle} training data set from UCI Machine Learning Repository \cite{UCI2013} contains $43,500$ points. We run  robust $k$-means++ on the \texttt{Shuttle} dataset with $k\in \{5, 10, 15\}$, and $\delta=\{0.05, 0.1\}.$ We compare its performance with vanilla $k$-means++ and random initialization. We summarise our empirical findings in Tables~\ref{tab:real11}, \ref{tab:real12}, \ref{tab:real13}, \ref{tab:real14}.

\paragraph{Insight.}  We notice that in almost every scenario robust $k$-means++ outperforms random initialization.  On the comparison with  $k$-means++ our algorithm gives  comparable/better  cost for all values of $k$. Specifically, our average cost is better than $k$-means++ on most of the instances. Our running time is slower albeit comparable to that of $k$-means++.
 
\begin{table}[ht]
%\begin{minipage}[b]{0.5\linewidth} 
% \caption*{\footnotesize{Robust $k$-means++ on~\texttt{Shuttle} dataset with  $k=5$ }}
 \scalebox{0.9}{
 \begin{tabular}{SlSSSSSSS}
    \toprule
    {Result}&
    \multirow{1}{*}{$\alpha$} &
      \multicolumn{3}{c}{Cost} &
      \multicolumn{3}{c}{Time(s)} \\
            &{}& {Min} & {Mean} & {Med.} & { } \\ 
      \midrule
                         
\text{This work}&$0$   &1.86 & \textbf{~~2.1} & \textbf{~~2.02}& 9.5 \\  
$\delta$=0.05	&$0.25$   &1.90 & \textbf{~~2.08} & \textbf{~~2.02}& 9.5 \\  
			&$0.5$   &1.85 & \textbf{~~2.06} & \textbf{~~2.02}& 9.5 \\ 
			&$0.75$   &\textbf{~~1.69} & \textbf{~~2.02} & \textbf{~~2.00}& 9.5 \\ 
			&$1$   &2.46 & 2.86 & 2.60& 9.5 \\ 
\hline			
\text{This work}&$0$   &1.87 & \textbf{~~2.08} & \textbf{~~2.02}& 5.3 \\  
$\delta$=0.1	&$0.25$   &1.85 & \textbf{~~2.04} & \textbf{~~2.01}& 5.3 \\  
			&$0.5$   &1.85 & \textbf{~~2.07} & \textbf{~~2.01}& 5.3 \\ 
			&$0.75$   &\textbf{~~1.66} & \textbf{~~2.08} & \textbf{~~2.03}& 5.3 \\ 
			&$1$   &2.24 & 2.67 & 2.60& 5.3\\			
			
          \hline      
     Min  $~\delta=0.05$ &  $$  &1.45     &1.75     &1.67         &5.4\\
     Min  $~\delta=0.1$ &  $$  &1.44     &1.92     &1.83         &5.4\\
           \hline
     
      $\kmpp$&  $$  &1.8     &2.4      &2.36         & 1.6  \\     
       \hline
      $\rand$&  $$  &2.6     &2.9      & 2.61         & 0.74 \\
    \bottomrule
  \end{tabular}
  }
  \vspace{-0.3cm}
  \caption{\footnotesize{Robust $k$-means++ on~\texttt{Shuttle} dataset with  $k=5$.
   We  delete the farthest $21$ points.  All cost are multiplicative of $10^8$.}}\label{tab:real11}
% \end{table}
%\end{minipage}
%\hspace{0.3cm}
%\begin{minipage}[b]{0.5\linewidth}
%\caption*{\footnotesize{Robust $k$-means++ on~\texttt{Shuttle} dataset with  $k=1$}}
\vspace{0.3cm}
  \scalebox{0.9}{
 \begin{tabular}{SlSSSSSSS}
    \toprule
    {Result}&
    \multirow{1}{*}{$\alpha$} &
      \multicolumn{3}{c}{Cost} &
      \multicolumn{3}{c}{Time(s)} \\
            &{}& {Min} & {Mean} & {Med.} & { } \\ 
      \midrule
                         
\text{This work}&$0$   &8.1 &\textbf{~~8.87} & \textbf{~~8.92}& 22.4 \\  
$\delta$=0.05	&$0.25$   &7.89 & \textbf{~~8.79} & \textbf{~~8.67}& 22.4 \\  
			&$0.5$   &\textbf{~~6.99}&\textbf{~~8.58} & \textbf{~~8.76}& 22.4 \\ 
			&$0.75$   &\textbf{~~6.67} & \textbf{~~8.56} & \textbf{~~8.56}& 22.4 \\ 
			&$1$   &9.47 &~~12.4 &~~12.6& 22.4 \\ 
\hline			
\text{This work}&$0$   &7.73 & \textbf{~~8.89} & \textbf{~~8.69}& 11.5 \\  
$\delta$=0.1	&$0.25$   &\textbf{~~6.8} & \textbf{~~8.86} & 9.11& 11.5 \\  
			&$0.5$   &\textbf{~~6.98} & \textbf{~~8.54} & \textbf{~~8.58}& 11.5 \\ 
			&$0.75$   &\textbf{~~6.95} & \textbf{~~8.31} & \textbf{~~8.11}& 11.5 \\ 
			&$1$   &9.72 &~~12 &~~12.6& 11.5\\			
			
           \hline   
           Min  $~\delta=0.05$ &  $$  &5.53     &6.78     &6.68         &5.4\\
           Min  $~\delta=0.1$ &  $$  &5.66     &6.59     &6.30         &5.4\\
           \hline
     
      $\kmpp$&  $$  &7.12&8.94&9.08&3.5\\     
       \hline
      $\rand$&  $$  &9.66 &11.6 &11.3&1.37 \\ 
    \bottomrule
  \end{tabular}
  }
  \vspace{-0.3cm}
\caption{\footnotesize{Robust $k$-means++ on~\texttt{Shuttle} dataset with  $k=10$. We  delete the farthest $34$ as outliers.
 All cost are multiplicative of $10^7$. }}\label{tab:real12}
\end{table}

\begin{table}[ht]
   \scalebox{0.9}{
 \begin{tabular}{SlSSSSSSS}
    \toprule
    {Result}&
    \multirow{1}{*}{$\alpha$} &
      \multicolumn{3}{c}{Cost} &
      \multicolumn{3}{c}{Time(s)} \\
            &{}& {Min} & {Mean} & {Med.} & { } \\ 
      \midrule
                         
\text{This work}&$0$   &\textbf{~~6.2}&\textbf{~~7.2}&\textbf{~~7.15}&37.5 \\  
$\delta$=0.05	&$0.25$   &\textbf{~~6.6}&\textbf{~~7.43}&\textbf{~~7.19}&37.5 \\  
			&$0.5$   &\textbf{~~6.05} &\textbf{~~7.26} &\textbf{~~7.18}& 37.5 \\ 
			&$0.75$   &\textbf{~~6.16} &\textbf{~~7.74} &\textbf{~~7.71}& 37.5 \\ 
			&$1$   &~~12.6 &~~17.9 &~~18.3& 37.5 \\ 
\hline			
\text{This work}&$0$   &\textbf{~~6.24} &\textbf{~~7.54}&\textbf{~~7.37}& 19.5 \\  
$\delta$=0.1	&$0.25$   &\textbf{~~6.34} &\textbf{~~7.22}& \textbf{~~7.14}& 19.5 \\  
			&$0.5$   &\textbf{~~6.37} &\textbf{~~7.68}& \textbf{~~7.69}& 19.5 \\ 
			&$0.75$   &\textbf{~~5.82} &\textbf{~~7.27}& \textbf{~~7.32}& 19.5 \\ 
			&$1$   &~~12.2 &~~19.4 &~~19.2& 19.5\\			
			
          \hline   
          Min  $~\delta=0.1$ &  $$  &5.52     &6.19     &5.94         &5.4\\
           Min  $~\delta=0.1$ &  $$  &5.11     &6.17     &6.08         &5.4\\
           \hline
     
      $\kmpp$&  $$  &6.78     &8.22     &8.01         &5.4\\     
       \hline
      $\rand$&  $$  &~~14.1    &~~16.3     &~~15.1         &1.98 \\ 
    \bottomrule
  \end{tabular}
  }
  \vspace{-0.3cm}
\caption{\footnotesize{Robust $k$-means++ on~\texttt{Shuttle} dataset with  $k=15$. We  delete the farthest $17$ as outliers.
 All cost are multiplicative of $10^7$.}}\label{tab:real13}
\vspace{0.3cm}
 
   \scalebox{0.9}{
 \begin{tabular}{SlSSSSSSS}
    \toprule
    {Result}&
    \multirow{1}{*}{$\alpha$} &
      \multicolumn{3}{c}{Cost} &
      \multicolumn{3}{c}{Time(s)} \\
            &{}& {Min} & {Mean} & {Med.} & { } \\ 
      \midrule
                         
\text{This work}&$0$   &4.2&4.94&4.91&37.5 \\  
$\delta$=0.05	&$0.25$   &4.2&5&5.03&37.5 \\  
			&$0.5$   &4.41 &5.04 &4.84& 37.5 \\ 
			&$0.75$   &4.21 &4.99 &4.94& 37.5 \\ 
			&$1$   &3.94 &4.98 &4.93& 37.5 \\ 
\hline			
\text{This work}&$0$   &4.13 & 4.96 & 5.01& 19.5 \\  
$\delta$=0.1	&$0.25$   &4.54 & 5.09 & 5.07& 19.5 \\  
			&$0.5$   &4.29 & 4.92 & 4.90& 19.5 \\ 
			&$0.75$   &4.13 &\textbf{~~4.56} & \textbf{~~4.57}& 19.5 \\ 
			&$1$   &4.22 & 5.28 & 5.37& 19.5\\			
			
          \hline      
    Min  $~\delta=0.05$ &  $$  &3.46     &3.96     &4.02         &5.4\\          
     Min  $~\delta=0.1$ &  $$  &3.07     &3.52     &3.44         &5.4\\
     \hline
      $\kmpp$&  $$  &3.89     &4.58     &4.57         &5.4\\     
       \hline
      $\rand$&  $$  &3.10    &4.91     &5.34         &2.02 \\ 
    \bottomrule
  \end{tabular}
  }
  \vspace{-0.3cm}
\caption{\footnotesize{Robust $k$-means++ on~\texttt{Shuttle} dataset with  $k=15$. We  delete the farthest $51$ as outliers.
 All cost are multiplicative of $10^7$. }}\label{tab:real14}
\end{table}

\subsection{Result on Synthetic  datasets} 
We recall the dataset generation step as follows. We pick $k + z$ uniformly random points from a large $d$-dimensional hypercube of side length $s = 100$. We use $k$ points from them as means and pick $n/k$ points around each of them from a random Gaussian of unit variance. This gives a data set of $n+z$ points with $n$ points clustered into $k$  clusters and the remaining $z$ as outliers.   We first run robust $k$-means++  with the values of   $\alpha\in\{0, 0.25, 0.5, 1\}$, $\delta\in\{0.05, 0.1\}$  on the synthetic datasets with values $n=1000, d=2, k=20$, and the number of outliers $\{25, 50, 120\}$.  We summarised our results in Tables~\ref{tab:synthetic10},\ref{tab:synthetic11},\ref{tab:synthetic12}.

\paragraph{Insight.}  We notice that in almost every scenario robust $k$-means++ outperforms random initialization.  On the comparison with  $k$-means++ our algorithm offers better performance in all the metric -- \texttt{min}, \texttt{mean}, \texttt{med} cost -- on all possible values of  $k, \alpha, \delta$.   Our running time is slower albeit comparable to that of $k$-means++.

%%%%%%%%%%%%%%%%%% SYNTHETIC DATASET RESULTS %%%%%%%%%%%%%%%%%%%%%
\setlength{\tabcolsep}{1.5pt}
\begin{table}[ht]
   \scalebox{0.9}{
 \begin{tabular}{SlSSSSSSS}
    \toprule
    {Result}&
    \multirow{1}{*}{$\alpha$}&
      \multicolumn{3}{c}{Cost}&
      \multicolumn{3}{c}{Time(s)}\\
            &{}&{Min}&{Mean}&{Med.}&{}\\ 
      \midrule
                         
\text{This work}&$0$ &\textbf{2035}&\textbf{2816}&\textbf{2733}&12 \\  
$\delta$=0.05	&$0.25$&2719&\textbf{3099}&\textbf{3272}&12 \\  
			&$0.5$ &\textbf{2036}&\textbf{2766}&\textbf{2581}&12 \\ 
			&$0.75$&\textbf{2543}&\textbf{3101}&\textbf{2927}& 12 \\ 
			&$1$   &\textbf{1996}&\textbf{2297}&\textbf{2298}&12 \\ 
\hline			
\text{This work}&$0$   &\textbf{2547} &\textbf{2834}&\textbf{2666}& 6.5 \\  
$\delta$=0.1	&$0.25$   &\textbf{2031} &\textbf{2737}& \textbf{2577}& 6.5 \\  
			&$0.5$   &\textbf{2542} &\textbf{2959}& \textbf{3072}& 6.5 \\ 
			&$0.75$   &\textbf{2032} &\textbf{2408}& \textbf{2297}& 6.5 \\ 
			&$1$   &\textbf{1907}&\textbf{2069}&\textbf{2037}& 6.5\\						
          \hline     
     Min$(\delta=0.1 )$&  $$  &1899&1951&1955&0.2\\   
      Min$(\delta=0.05 )$&  $$  &1907&1953&1957&0.2\\  
      $\kmpp$&  $$  &2561&4840&4145&0.2\\     
       \hline
      $\rand$&  $$  &5443&17977&13753&0.07 \\ 
    \bottomrule
  \end{tabular}
  }
  \vspace{-0.3cm}
\caption{\footnotesize{Robust $k$-means++ on Synthetic dataset with $\delta=0.1$. $n = 1000, d = 2, k = 20.$ We delete the farthest $25$ as outliers.}}\label{tab:synthetic10}
\vspace{0.3cm}
\end{table}
%%%%%%%%%%%%%%%
\begin{table}[ht]
   \scalebox{0.9}{
 \begin{tabular}{SlSSSSSSS}
    \toprule
    {Result}&
    \multirow{1}{*}{$\alpha$} &
      \multicolumn{3}{c}{Cost} &
      \multicolumn{3}{c}{Time(s)} \\
            &{}&{Min} &{Mean} &{Med.} & { } \\ 
      \midrule
                         
\text{This work}&$0$ &\textbf{1880}&\textbf{1907}&\textbf{1912}&12 \\  
$\delta$=0.05	&$0.25$&1890&\textbf{1908}&\textbf{1906}&12 \\  
			&$0.5$ &1884&\textbf{1909}&\textbf{1904}&12 \\ 
			&$0.75$&1892&\textbf{1921}&\textbf{1908}& 12 \\ 
			&$1$   &\textbf{1753}&\textbf{1879}&\textbf{1893}&12 \\ 
\hline			
\text{This work}&$0$   &1882 &\textbf{1927}&\textbf{1914}& 6.5 \\  
$\delta$=0.1	&$0.25$   &1892 &\textbf{1908}& \textbf{1906}& 6.5 \\  
			&$0.5$   &1891 &\textbf{1902}& \textbf{1896}& 6.5 \\ 
			&$0.75$   &1883 &\textbf{1905}& \textbf{1899}& 6.5 \\ 
			&$1$   &\textbf{1746}&\textbf{1855}&\textbf{1887}& 6.5\\			
			
          \hline      
      Min $(\delta=0.1)$&  $$  &2211     &2731     &2310         &0.2\\ 
      Min $(\delta=0.05)$&  $$  &2211     &2707     &2993         &0.2\\
      \hline
      $\kmpp$&  $$  &1881     &6113     &5011         &0.2\\     
       \hline
      $\rand$&  $$  &8939    &28696     &27168         &0.07 \\ 
    \bottomrule
  \end{tabular}
  }
  \vspace{-0.3cm}
\caption{\footnotesize{Robust $k$-means++ on Synthetic dataset with $\delta=0.1$. $n = 1000, d = 2, k = 20.$ We delete the farthest $50$ as outliers.}}\label{tab:synthetic11}
\vspace{0.3cm}
\end{table}
%%%%%%%%%%%%%%%%%%%

\begin{table}[ht]
   \scalebox{0.9}{
 \begin{tabular}{SlSSSSSSS}
    \toprule
    {Result}&
    \multirow{1}{*}{$\alpha$} &
      \multicolumn{3}{c}{Cost} &
      \multicolumn{3}{c}{Time(s)} \\
            &{}&{Min} &{Mean} &{Med.} & { } \\ 
      \midrule
                         
\text{This work}&$0$ &3313&\textbf{5135}&\textbf{5010}&12 \\  
$\delta$=0.05	&$0.25$&3283&\textbf{4572}&\textbf{4480}&12 \\  
			&$0.5$ &4249&\textbf{4808}&\textbf{4649}&12 \\ 
			&$0.75$&2514&\textbf{4647}&\textbf{4449}& 12 \\ 
			&$1$   &\textbf{2016}&\textbf{2780}&\textbf{2592}&12 \\ 
\hline			
\text{This work}&$0$   &3538 &\textbf{4975}&\textbf{4673}& 6.5 \\  
$\delta$=0.1	&$0.25$   &3306 &\textbf{4064}& \textbf{4178}& 6.5 \\  
			&$0.5$   &3284&\textbf{4293}& \textbf{4146}& 6.5 \\ 
			&$0.75$   &2737 &\textbf{3686}& \textbf{3554}& 6.5 \\ 
			&$1$   &\textbf{1779}&\textbf{2656}&\textbf{2657}& 6.5\\			
			
          \hline      
     Min $(\delta=0.1)$&  $$  &1908     &3315     &3011         &0.2\\   
    Min $(\delta=0.05)$&  $$  &1933     &3525     &3777         &0.2\\   
     \hline
      $\kmpp$&  $$  &2188     &6272     &6053         &0.2\\     
       \hline
      $\rand$&  $$  &7428    &22902     &21449         &0.07 \\ 
    \bottomrule
  \end{tabular}
  }
  \vspace{-0.3cm}
\caption{\footnotesize{Robust $k$-means++ on Synthetic dataset with $\delta=0.1$. $n = 1000, d = 2, k = 20.$ 
We delete the farthest $120$ as outliers.}}\label{tab:synthetic12}
\vspace{0.3cm}
\end{table}
